# Supplementary material for: Image Watermarking With Memory Across Reissuance
Source: arXiv:2611.23363 source file (2026-11-17)
Supplement: Supplementary file 1 [file appendix_snapshot_controls.tex]

\section{Evaluation Instantiation}
\label{app:evaluation-instantiation}

\paragraph{Spatial carrier.}
Images are evaluated at $512\!\times\!512$ resolution on a
$16\!\times\!16$ grid of $32\!\times\!32$-pixel cells.  Of the 256 cells, 32
carry lineage evidence, 64 carry issue evidence, and 160 carry the keyed
two-bit generation field.  Cell allocation, writer and reader weights,
decision thresholds, prompts, editor assignment, and random seeds are frozen
before the 480-root evaluation.

\paragraph{Authorized-scope instantiation.}
Because the instruction-based editors do not expose a native revision mask,
the experiment constructs the scope proposal directly from the spatial cells
in which the complete editor output disrupts the registered parent's
watermark.  A frozen watermark-damage score is thresholded at $Q_{0.75}$ and
expanded by at most eight grid iterations to a minimum support of 32 cells.
This disruption-derived proposal becomes $A_g$ only when the simulated issuer
authenticates it at commitment; unissued editor outputs do not advance the
generation field.

\paragraph{Image fidelity.}
For the 480 initial protected issues, PSNR relative to the unprotected root
has median 46.69 dB, tenth percentile 42.50 dB, and minimum 36.85 dB.

\section{Complete-Output Protocol Controls}
\label{app:complete-output-controls}

\paragraph{Snapshot localizers under native and retained-output endpoints.}
The main evaluation retains every editor-returned RGB image.  To isolate the
consequence of this choice, we run EditGuard and OmniGuard on 1,000 matched
edits under both their native inpainting/paste-back endpoint and the
complete-output endpoint.  Under the native endpoint, the protected pixels
outside the edited region are copied back unchanged.  Under the retained
endpoint, the localizer receives the editor's complete output, exactly as in
the reissuance trajectories.

\begin{center}
\refstepcounter{table}\label{tab:complete-output-control}
\begin{minipage}{\columnwidth}
\small
\noindent Table~\thetable: Matched snapshot-localization control.  Predicted
area is the positive fraction of the complete-output mask.  Values are
percentages.
\par\smallskip
\centering
\resizebox{\linewidth}{!}{%
\begin{tabular}{lccc}
\toprule
Method & Native F1 & Complete predicted area & Complete F1 \\
\midrule
EditGuard & 97.18 & 100.00 & 16.81 \\
OmniGuard & 98.47 & 0.27 & 0.00 \\
\bottomrule
\end{tabular}}
\end{minipage}
\end{center}

Both methods remain strong at their native endpoint.  Retaining the complete
image changes the physical observation: EditGuard expands to an all-positive
mask, while OmniGuard collapses to a near-empty mask.  This is consistent with
the median changed-cell fraction of 1.00 for all four complete-output editors.
The control establishes that a complete generative return is not equivalent
to inpainting followed by copying an unchanged protected background.

This comparison is a protocol control rather than a ranking on the same
semantic task.  Snapshot localization asks which part of one protected image
was disrupted.  Reissuable provenance begins with the subsequent event: the
retained image is \textsc{Open} until authorization, and a fresh complete
embedding carries the authorized result forward as a new issue with
head-relative state and inherited regional history.

\section{Generation-Specific Map Accuracy}
\label{app:generation-specific-iou}

Table~\ref{tab:generation-specific-iou} separates the macro result in
Table~\ref{tab:generation-map-results} by temporal label.  Each entry is the median
IoU over successors in which that generation is present.  The newest label is
also the current-scope IoU reported in the main paper; the earlier columns
measure historical spatial attribution.

\begin{center}
\refstepcounter{table}\label{tab:generation-specific-iou}
\begin{minipage}{\columnwidth}
\small
\noindent Table~\thetable: Generation-specific IoU of the spatial reader.
Entries are percentages; dashes denote labels that do not yet exist.
\par\smallskip
\centering
\begin{tabular}{crrrr}
\toprule
Depth & Generation 0 & Generation 1 & Generation 2 & Generation 3 \\
\midrule
1 & 93.99 & 94.92 & -- & -- \\
2 & 89.32 & 83.33 & 94.09 & -- \\
3 & 81.48 & 72.57 & 81.32 & 92.86 \\
\bottomrule
\end{tabular}
\end{minipage}
\end{center}

\section{Rendition-Wise Lifecycle Robustness}
\label{app:rendition-robustness}

Table~\ref{tab:rendition-full} expands the 22-world family-level median and
minimum summary in Table~\ref{tab:open-robustness} into the complete per-world
results.  It also
reports both sides of the carrier tradeoff: unissued outputs retain high
\textsc{Open} recall because issue discontinuity remains visible, while severe
re-encoding can erase the positive evidence required to accept an issued image
as \textsc{Current}.  This is why \textsc{Open} robustness and current-issue
retention are reported as separate quantities.

\begin{center}
\refstepcounter{table}\label{tab:rendition-full}
\begin{minipage}{\textwidth}
\scriptsize
\noindent Table~\thetable: Per-world lifecycle results.  $O_0$ is
\textsc{Open} recall at the initial edit; $O_{T/B}$ combines terminal and
branch outputs.  $C_0$ and $C_3$ are \textsc{Current} accuracy for the initial
and final registered issues.  All entries are percentages.
\par\smallskip
\centering
\resizebox{\textwidth}{!}{%
\begin{tabular}{lrrrr@{\qquad}lrrrr}
\toprule
World & $O_0$ & $O_{T/B}$ & $C_0$ & $C_3$ &
World & $O_0$ & $O_{T/B}$ & $C_0$ & $C_3$ \\
\midrule
Clean                    & 96.04 & 93.12 & 99.58 & 98.96 &
JPEG 30                  & 99.38 & 99.58 &  0.00 &  0.00 \\
Brightness $\times0.85$  & 95.62 & 94.06 & 99.58 & 99.38 &
Resize 320               & 96.88 & 95.94 & 99.58 & 98.96 \\
Brightness $\times1.15$  & 97.71 & 93.85 & 45.42 & 72.50 &
Resize 256               & 96.67 & 94.58 & 99.58 & 99.38 \\
Contrast $\times0.80$    & 94.17 & 93.44 & 99.17 & 99.17 &
Resize 192               & 99.17 & 97.60 &  0.42 &  1.04 \\
Contrast $\times1.25$    & 97.29 & 93.33 & 26.04 & 64.58 &
Blur $\sigma=0.5$        & 96.67 & 93.85 & 99.58 & 98.96 \\
Gamma $0.80$             & 95.21 & 92.92 & 69.38 & 75.00 &
Blur $\sigma=1.0$        & 97.29 & 96.56 & 99.58 & 98.12 \\
Gamma $1.25$             & 96.46 & 93.96 & 59.79 & 66.67 &
Double JPEG 75           & 97.71 & 96.77 & 94.17 & 95.21 \\
JPEG 75                  & 98.33 & 96.46 & 96.67 & 95.62 &
Platform A               & 99.17 & 98.33 & 44.79 & 58.13 \\
Resize 384               & 95.62 & 94.17 & 99.79 & 99.38 &
Platform B               & 99.38 & 99.27 &  0.62 &  2.50 \\
JPEG 50                  & 99.38 & 98.75 & 38.75 & 35.00 &
Brightness $\times1.30$  & 98.12 & 95.73 & 15.21 & 39.38 \\
JPEG 40                  & 99.79 & 99.38 &  4.17 &  1.67 &
Contrast $\times1.50$    & 96.67 & 95.21 &  6.88 & 31.25 \\
\bottomrule
\end{tabular}}
\end{minipage}
\end{center}

\paragraph{Carrier retention.}
Sufficiently destructive re-encoding can erase the positive evidence of a
truly current issue and move the verifier toward \textsc{Open} or
\textsc{Unknown}.  The $C_0$ and $C_3$ columns above quantify this physical
retention limit separately from event-defined lifecycle truth.  It affects
evidence observability, not the authorization graph or the fresh-reissuance
transition.
